# Supplementary material for: QPack: Quantum Approximate Optimization Algorithms as universal benchmark for quantum computers
Source: arXiv:2103.17193 source file (2022-04-19)
Supplement: Supplementary file 1 [file code_appendix.tex]

\section{Code implementations}

\subsection{MCP implementation} \label{app:mcp-qiskit}
\lstset{
  basicstyle=\footnotesize, frame=tb,
  xleftmargin=0.0\textwidth, xrightmargin=.2\textwidth
}
\begin{lstlisting}
# circuit definition for QAOA MaxCut
def max_cut_circ(params, graph, p, backend):
    beta = params[0:p]
    gamma = params[p:2*p]

    v, edge_list = graph
    vertice_list = list(range(0, v, 1))

    # initialise quantum circuit
    c = ClassicalRegister(v)
    q = QuantumRegister(v)
    qc = QuantumCircuit(q, c)
    
    # apply hadamard to each qubit
    for qubit in range(v):
        qc.h(qubit)
        
    #apply cost and mixer uinitary for each layer of p
    for iteration in range(p):
        for e in edge_list:
            qc.cnot(e[0], e[1])
            qc.rz(-gamma[p-1], e[1])
            qc.cnot(e[0], e[1])
        for qb in vertice_list:
            qc.rx(2*beta[p-1], qb)
    qc.measure(q, c)
    job = execute(qc, backend, shots=qaoa_shots)
    result = job.result()
    out_state = result.get_counts()
    prob = list(out_state.values())
    states = list(out_state.keys())
    exp = 0
    for k in range(len(states)):
        exp += eval_cost(states[k], graph)*prob[k]
    return [exp/qaoa_shots]
\end{lstlisting}

\lstset{
  basicstyle=\footnotesize, frame=tb,
  xleftmargin=.0\textwidth, xrightmargin=.2\textwidth
}
\begin{lstlisting}
# cost evaluation for MaxCut
def eval_mcp(out_state, graph):
    v = graph[0]
    edges = graph[1]
    c = 0
    # convert values from outstate
    bin_val = [int(i) for i in list(out_state)]
    bin_val = [-1 if x == 0 else 1 for x in bin_val]
    # evaluate cost
    for e in edges:
        c += 0.5 * (1 - int(bin_val[e[0]]) 
        c = c * int(bin_val[e[1]]))
    return c
\end{lstlisting}

\subsection{DSP implementation}
\label{app:dsp-qiskit}
\begin{lstlisting}
def dsp_circuit(params, graph, p, backend):
# quantum circuit for dominating set
    beta = params[0:p]
    gamma = params[p:2*p]
    v, edge_list = graph
    vertice_list = list(range(0, v, 1))
    # initialise a list of the connections 
    # (list of nodes, connected to the node)
    connections = []
    for i in range(v):
        connections.append([i])
    for t in edge_list:
        connections[t[0]].append(t[1])
        connections[t[1]].append(t[0])
    ancillas = 0
    for con in connections:
        if len(con) > ancillas:
            ancillas = len(con)
    n = v+ancillas         # add ancillas
    qc = QuantumCircuit(n, v)

    # initialise with hadamard to each qubit
    for qubit in range(v):
        qc.h(qubit)
        # inverted  controlled rotation Z gate
        qc.x(qubit)
        qc.crz(-gamma[0], qubit, n-1)
        qc.x(qubit)
    # cost unitary and mixer unitary for 
    # QAOA layers (p)
    for iteration in range(p):
        f = 0
        f_anc = v
        for con in connections:
            c_len = len(con)
            # n-qubit controller rotation Z gate 
            # (OR_nrz)
            OR_range = con.copy()
            for k in range(c_len-1):
                OR_range.append(v+k)
            cOR_rz = OR_nrz(c_len, gamma[p-1])
            OR_range.append(n-1)
            qc.append(cOR_rz, OR_range)

        for qb in vertice_list:
            qc.rx(-2*beta[p-1], qb)
    qc.measure(range(v), range(v))
    job = execute(qc, backend, shots=qaoa_shots)
    result = job.result()
    out_state = result.get_counts()
    return out_state
\end{lstlisting}

\begin{lstlisting}
# cost evaluation dominating set
def dsp_cost(params, v, e, p, backend):
    graph = [v, e]
    beta = params[0:p]
    gamma = params[p:2*p]

    out_state = dsp_circuit(params, graph, p, backend)

    edge_list = e
    vertice_list = list(range(0, v, 1))
    connections = []
    for i in range(v):
        connections.append([i])
    for t in edge_list:
        connections[t[0]].append(t[1])
        connections[t[1]].append(t[0])
    total_count = 0
    total_cost = 0
    for p_it in out_state:
        for t in out_state:
            count = int(out_state.get(t))
            total_count += count
            bin_len = "{0:0" + str(v) + "b}"  # string required for binary formatting
            bin_val = t.format(bin_len)
            bin_val = [int(i) for i in bin_val]
            # cost T
            T = 0 (+1 if node not connected/dominated)
            for con in connections:
                tmp = 0
                for k in con:
                    tmp = tmp or bin_val[k]
                    if tmp:
                        T += 1
                        break
            # cost D (+1 for each node dominating)
            D = 0
            for i in range(v):
                D += 1 - bin_val[i]
            total_cost += (T+D)*count
    total_cost = total_cost/total_count
    return total_cost
\end{lstlisting}

\subsection{TSP implementation}
\label{app:tsp-qiskit}
\begin{lstlisting}
def tsp_circ(params, graph, p, rep, backend):
# QAOA circuit for TSP
    beta = params[0:p]
    gamma = params[p:2*p]
    v, A, D = graph

    vertice_list = list(range(0, v, 1))

    # initialize circuit
    n = v**2
    qc = QuantumCircuit(n, n)
    # initialization using the Dicke state preparation
    for q in range(v):
        q_range = range(q*v, (q+1)*v)
        DickeGate = dicke_init(v, 2)
        qc.append(DickeGate, q_range)
    # QAOA cycles
    # for 1 to p:

    # cost unitary
    for iteration in range(p):
        for i in range(n):
            qc.rz(gamma[p-1]*D[i]/(2*pi), i)

        for i in range(v):
            for j in range(i):
                if i != j:
                    qc.rzz(20*gamma[p-1]/pi, (j+i*v), i+j*v)

        # mixer unitary
        for i in range(0, v):
            qc.rxx(-beta[p-1], i*v, (i*v+1))
            qc.rxx(-beta[p-1], (i*v+1), (i*v+2))

            qc.ryy(-beta[p-1], i * v, (i * v + 1))
            qc.ryy(-beta[p-1], (i * v + 1), (i * v + 2))

        qc.measure(range(n), range(n))
        job = execute(qc, backend, shots=rep)
        result = job.result()
        out_state = result.get_counts()
    return out_state
\end{lstlisting}

\begin{lstlisting}
# TSP cost evaluation
def cost_tsp(params, graph, p, rep, backend):
    v, A, D = graph
    # measured state formatting
    out_state = tsp_circ(params, graph, p, rep, backend)
    total_cost = 0
    coupling = []
    for i in range(v):
        for j in range(i):
            if i != j:
                coupling.append([i + j * v, j + i * v])
    for t in out_state:
        count = int(out_state.get(t))
        bin_len = "{0:0" + str(v) + "b}"  # string required for binary formatting
        bin_val = t.format(bin_len)
        bin_val = [int(i) for i in bin_val]
        # cost evaluation
        cost = 0
        for i in range(0, v):
            for j in range(0, v):
                cost += 0.5*D[i + v*j]*bin_val[i + v*j]
        for j in coupling:
            cost += -5*(1 - 2*bin_val[j[0]])*(1 - 2*bin_val[j[1]])
        total_cost += (cost*count)/rep
    return total_cost
\end{lstlisting}

\subsection{Additional quantum gates} \label{app:a}
This appendix contains an overview of omitted gates, used in the implementation of the QAOA circuits for the dominating set and traveling salesman.

\begin{lstlisting}
# controlled rotation Y
def cry(theta):
    qc = QuantumCircuit(2)
    qc.ry((pi/2)-theta/2, 0)
    qc.cnot(1, 0)
    qc.ry(-((pi/2)-theta/2), 0)
    return qc.to_gate()
\end{lstlisting}

\begin{lstlisting}
# 2-qubit controlled rotation Y
def ccry(theta):
    qc = QuantumCircuit(3)
    qc.toffoli(0, 1, 2)
    qc.ry(-theta/2, 2)
    qc.toffoli(0, 1, 2)
    qc.ry(theta / 2, 2)
    return qc.to_gate()
\end{lstlisting}

\begin{lstlisting}
# Split & Cyclic Shift unitary (SCS) gate
def scs(n, k):
    qc = QuantumCircuit(n)
    qc.cnot(n - 2, n-1)
    theta = 2 * (acos(sqrt(1 / n)))
    qc.append(cry(theta), [n-2, n - 1])
    qc.cnot(n - 2, n-1)

    for m in range(k - 1):
        l = 2+m
        control = n-2-m
        qc.cnot(control-1, n-1)
        theta = 2 * (acos(sqrt((n-control) / n)))
        qc.append(ccry(theta), 
            [n-1, control, control-1])

        qc.cnot(control-1, n-1)
    return qc.to_gate()
\end{lstlisting}

\begin{lstlisting}
#deterministic  Dicke state preparation (Bartschi & Eidenbenz, 2019)
def dicke_init(n, k):
    #unoptimized version
    qc = QuantumCircuit(n)
    qc.x(range(n-k, n))
    for i in range(n, k, -1):
        qc.append(scs(i, k), range(0, i))

    for i in range(k, 1, -1):
        qc.append(scs(i, i-1), range(0, i))

    return qc.to_gate()
\end{lstlisting}

\begin{lstlisting}
# 2-qubit OR gate
def OR_2q():
    qc = QuantumCircuit(3)
    qc.toffoli(0, 1, 2)
    qc.cnot(0, 1)
    qc.cnot(0, 2)
    return qc.to_gate()
\end{lstlisting}

\begin{lstlisting}
# n-qubit controlled rotation Z gate
def OR_nrz(n, gamma):
    ORGate = OR_2q()
    qc = QuantumCircuit(2*n)
    qc.append(ORGate, [0, 1, n])
    for i in range(2, n):
        qc.append(ORGate, [i, n+i-2, n+i-1])
    qc.crz(gamma, 2*n-2, 2*n-1)
    for i in range(n, 2, -1):
        qc.append(ORGate, [n-i-1, 2*n-2-i, 2*n-1-i])
    qc.append(ORGate, [0, 1, n])
    return qc.to_gate()
\end{lstlisting}
